# Supplementary material for: Diagnostics of Data-Driven Models: Uncertainty Quantification of PM7 Semi-Empirical Quantum Chemical Method
Source: arXiv:1806.04813 ancillary file (2018-06-16)
Supplement: Supplementary file 1 [file supporting-information.pdf]

# Supporting Information - Diagnostics of Data-Driven Models: Uncertainty Quantification of PM7 Semi-Empirical Quantum Chemical Method

James Oreluk*, Zhenyuan Liu*, Arun Hegde*, Wenyu Li*, Andrew Packard*, Michael Frenklach†, Dmitry Zubarev‡

June 16, 2018

Feasible parameter vectors and feasibility labels data are available from the authors upon request.

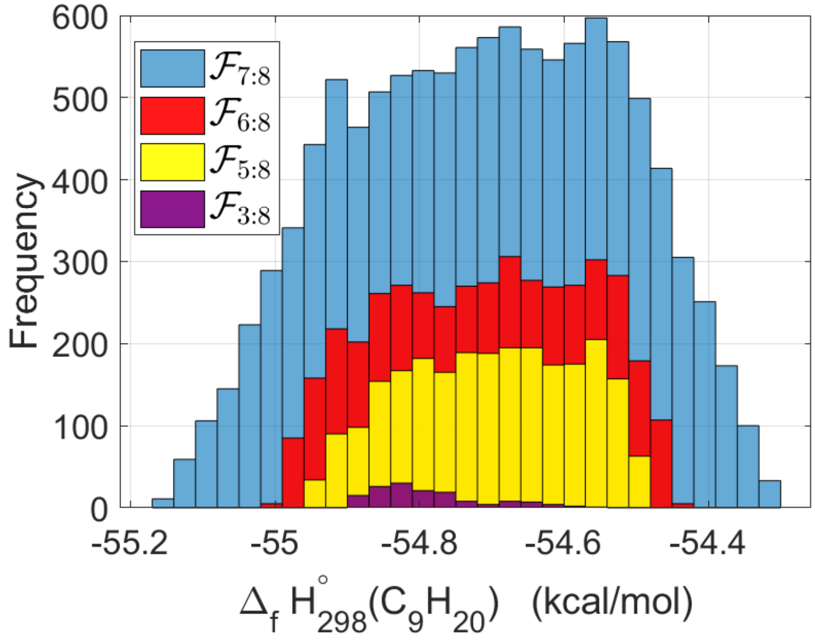


Figure S1: Predicted heat of formation of nonane by feasible samples of smaller alkanes. Using samples of $\mathcal{F}_{3:8}$ reduce the uncertainty in the predicted heat of formation by 40.5% compared to the prediction from samples of $\mathcal{F}_{7:8}$.

*Department of Mechanical Engineering, University of California at Berkeley, Berkeley, California 94720-1740

†Corresponding author: frenklach@berkeley.edu, Department of Mechanical Engineering, University of California at Berkeley, Berkeley, California 94720-1740

‡IBM Almaden Research Center, 650 Harry Road, San Jose, California 95136

Table S1: PM7 nominal parameter vector and the $\delta$ associated with a 10 kcal/mol change in the heat of formation of $C_4H_{10}$, where each parameter value was perturbed, one-at-a-time from its nominal value.

| **Parameter** | **Value** | $\boldsymbol{\delta}$ |
|---|---|---|
| $\mathbf{USS_H}$ | -11.07 | 0.29033 |
| $\mathbf{BETAS_H}$ | -8.3897 | 0.069276 |
| $\mathbf{ZS_H}$ | 1.2602 | 0.017434 |
| $\mathbf{GSS_H}$ | 14.15 | 0.36839 |
| $\mathbf{FN11_H}$ | 0.17785 | 0.009959 |
| $\mathbf{FN21_H}$ | 1.4287 | 0.33716 |
| $\mathbf{FN31_H}$ | 0.99132 | 0.077376 |
| $\mathbf{ALPB_H}$ | 4.0512 | 0.54877 |
| $\mathbf{XFAC_H}$ | 2.8456 | 4.875 |
| $\mathbf{USS_C}$ | -51.373 | 0.11427 |
| $\mathbf{UPP_C}$ | -40.135 | 0.084482 |
| $\mathbf{BETAS_C}$ | -14.415 | 0.12922 |
| $\mathbf{BETAP_C}$ | -7.8937 | 0.067632 |
| $\mathbf{ZS_C}$ | 1.9422 | 0.012886 |
| $\mathbf{ZP_C}$ | 1.7087 | 0.007471 |
| $\mathbf{GSS_C}$ | 12.347 | 0.13671 |
| $\mathbf{GSP_C}$ | 11.933 | 0.18749 |
| $\mathbf{GPP_C}$ | 10.452 | 0.8254 |
| $\mathbf{GP2_C}$ | 9.3855 | 0.031369 |
| $\mathbf{HSP_C}$ | 0.80263 | 0.11697 |
| $\mathbf{FN11_C}$ | 0.045888 | 0.005604 |
| $\mathbf{FN21_C}$ | 5.0371 | 1.5601 |
| $\mathbf{FN31_C}$ | 1.5887 | 0.12723 |
| $\mathbf{ALPB_{HC}}$ | 1.0387 | 0.007624 |
| $\mathbf{XFAC_{HC}}$ | 0.20458 | 0.002002 |
| $\mathbf{ALPC_C}$ | 2.6557 | 0.024061 |
| $\mathbf{XFAC_C}$ | 0.93782 | 0.034605 |

Table S2: Parameter vector of $\mathcal{F}_{2:8}$ found via global optimization with a genetic algorithm using MATLAB's *ga* function.

| Parameter | Value |
|---|---|
| $\mathbf{USS_H}$ | -14.577 |
| $\mathbf{BETAS_H}$ | -7.3947 |
| $\mathbf{ZS_H}$ | 1.1558 |
| $\mathbf{GSS_H}$ | 15.096 |
| $\mathbf{FN11_H}$ | 0.21973 |
| $\mathbf{FN21_H}$ | 1.3555 |
| $\mathbf{FN31_H}$ | 0.89818 |
| $\mathbf{ALPB_H}$ | 4.0908 |
| $\mathbf{XFAC_H}$ | 2.6264 |
| $\mathbf{USS_C}$ | -50.896 |
| $\mathbf{UPP_C}$ | -42.679 |
| $\mathbf{BETAS_C}$ | -12.204 |
| $\mathbf{BETAP_C}$ | -8.0123 |
| $\mathbf{ZS_C}$ | 1.9807 |
| $\mathbf{ZP_C}$ | 1.5976 |
| $\mathbf{GSS_C}$ | 12.653 |
| $\mathbf{GSP_C}$ | 10.104 |
| $\mathbf{GPP_C}$ | 9.8942 |
| $\mathbf{GP2_C}$ | 9.8562 |
| $\mathbf{HSP_C}$ | 0.77597 |
| $\mathbf{FN11_C}$ | 0.051751 |
| $\mathbf{FN21_C}$ | 4.8582 |
| $\mathbf{FN31_C}$ | 1.6624 |
| $\mathbf{ALPB_{HC}}$ | 1.0878 |
| $\mathbf{XFAC_{HC}}$ | 0.17728 |
| $\mathbf{ALPC_C}$ | 2.5316 |
| $\mathbf{XFAC_C}$ | 0.75887 |

Table S3: Percentage of feasible points found (out of 5.76 million samples) for each alkane and pair of alkanes.

| | $CH_4$ | $C_2H_6$ | $C_3H_8$ | $C_4H_{10}$ | $C_5H_{12}$ | $C_6H_{14}$ | $C_7H_{16}$ | $C_8H_{18}$ |
|---|---|---|---|---|---|---|---|---|
| $CH_4$ | 0.2647 | 0.0036 | 0.0028 | 0.0027 | 0.0026 | 0.0019 | 0.0025 | 0.0030 |
| $C_2H_6$ | | 0.4253 | 0.0148 | 0.0113 | 0.0093 | 0.0077 | 0.0088 | 0.0100 |
| $C_3H_8$ | | | 0.4063 | 0.0318 | 0.018 | 0.0133 | 0.0140 | 0.0159 |
| $C_4H_{10}$ | | | | 0.4441 | 0.0572 | 0.0317 | 0.0297 | 0.0307 |
| $C_5H_{12}$ | | | | | 0.4172 | 0.0698 | 0.0501 | 0.0461 |
| $C_6H_{14}$ | | | | | | 0.3869 | 0.1070 | 0.0750 |
| $C_7H_{16}$ | | | | | | | 0.4723 | 0.1915 |
| $C_8H_{18}$ | | | | | | | | 0.5723 |

Table S4: Largest percentage of feasible samples for three alkanes, indexed by QOI model.

| $\mathcal{F}_{i,j,k}$ | **Percentage of feasible samples** |
|---|---|
| 6, 7, 8 | 0.0738 |
| 5, 6, 7 | 0.0488 |
| 5, 6, 8 | 0.0434 |
| 5, 7, 8 | 0.0432 |
| 4, 5, 6 | 0.0312 |
| 4, 5, 7 | 0.0285 |
| 4, 6, 7 | 0.0282 |
| 4, 5, 8 | 0.0278 |
| 4, 7, 8 | 0.0266 |
| 4, 6, 8 | 0.0260 |

Table S5: Feasible sets of consecutive alkanes which had a few or no feasible samples, indexed by the QOI model.

| **QOI Index** | **Number of feasible samples** |
|---|---|
| 1, 2, 3 | 7 |
| 1, 2, 3, 4 | 4 |
| 1, 2, 3, 4, 5 | 0 |
| 2, 3, 4, 5 | 7 |
| 5, 6, 7 | 2809 |
| 5, 6, 7, 8 | 2431 |
| 4, 5, 6, 7, 8 | 1431 |
| 3, 4, 5, 6, 7, 8 | 145 |

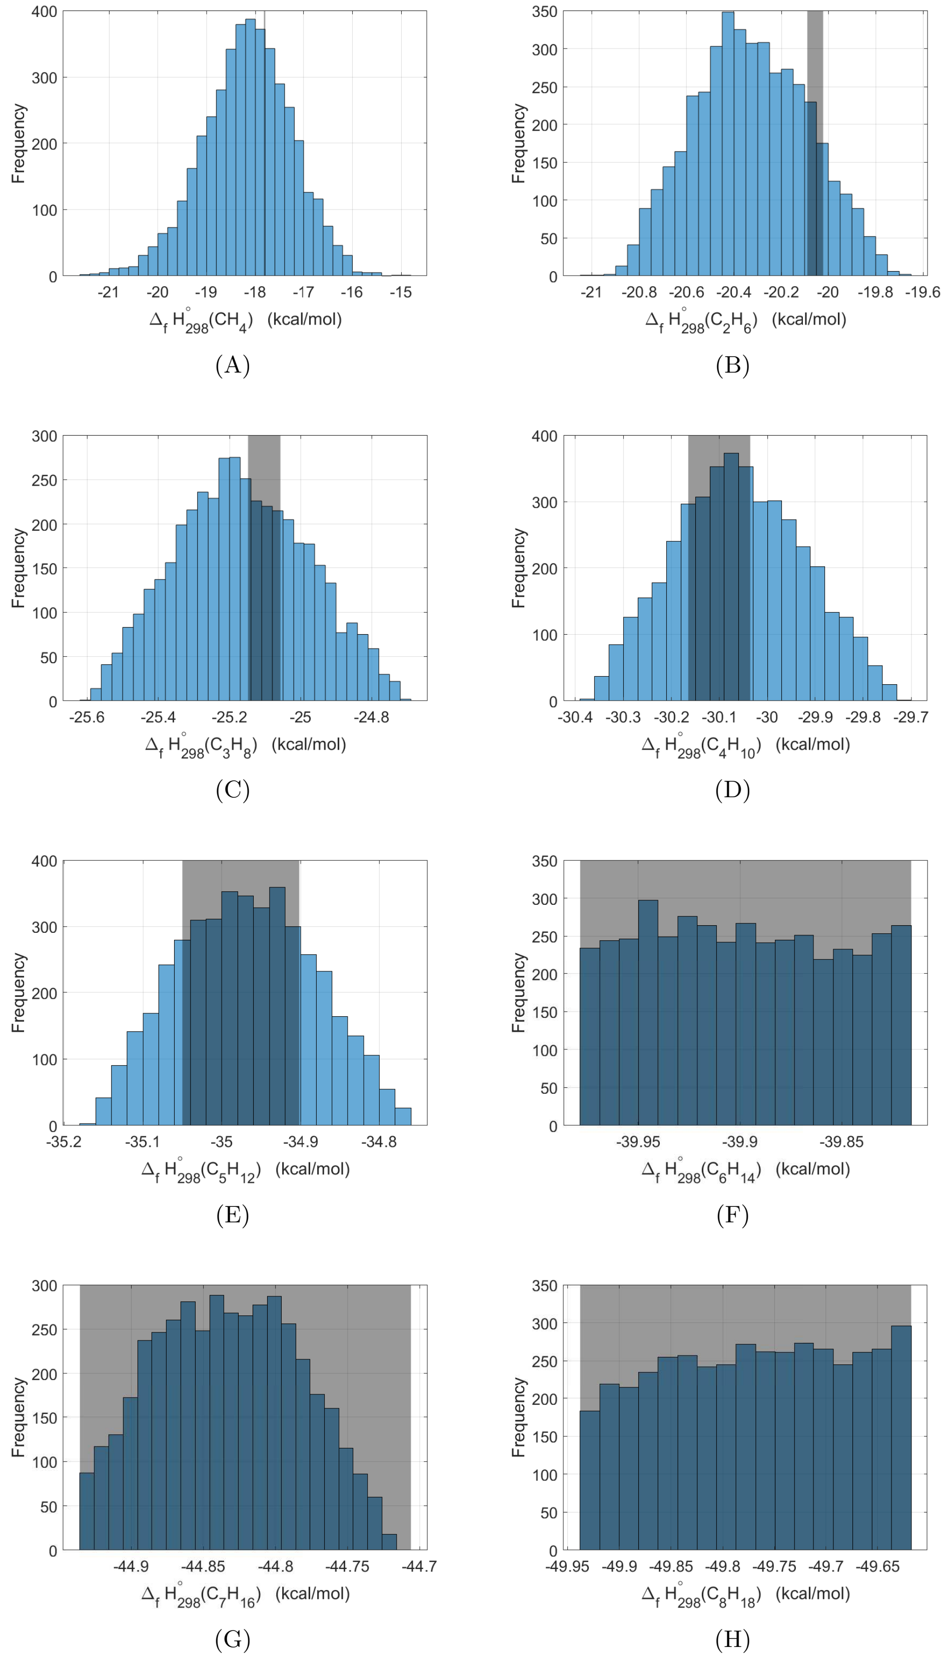


Figure S2: Predicted heat of formation of methane, ethane, to octane from samples of $\mathcal{F}_{6:8}$. The grey shaded region is the respective alkanes experimental interval shown in Table 1.

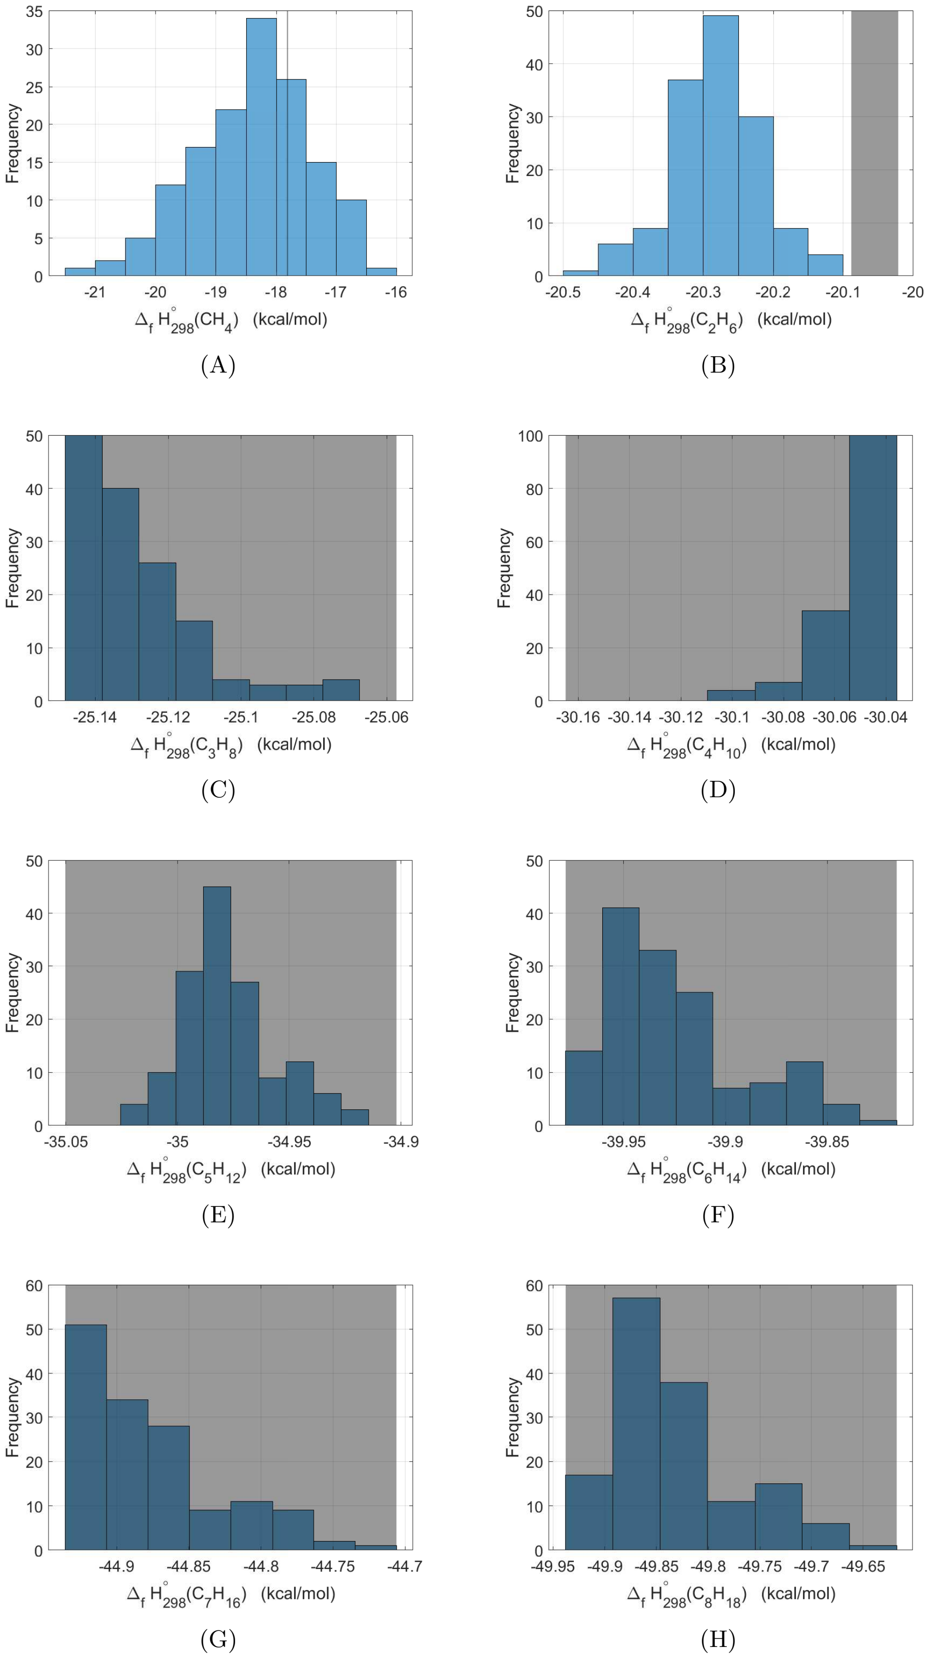


Figure S3: Predicted heat of formation of methane, ethane to octane from samples of $\mathcal{F}_{3:8}$. The grey shaded region is the respective alkanes experimental interval shown in Table 1.

## Acknowledgments

Work at UCB was supported by the Department of Energy, National Nuclear Security Administration, under Award Number(s) DE-NA0002375. The views and opinions of authors expressed herein do not necessarily state or reflect those of the United States Government or any agency thereof.
